# Supplementary material for: Modeling Player and Team Performance in Basketball
Source: arXiv:2007.10550 source file (2020-07-21)
Supplement: Supplementary file 1 [file supplement.tex]

\documentclass{article}

\usepackage[comma]{natbib}
\usepackage[margin=1in]{geometry}
\setcounter{secnumdepth}{4}

% Metadata Information
% \jname{Xxxx. Xxx. Xxx. Xxx.}
% \jvol{AA}
% \jyear{YYYY}
% \doi{10.1146/((please add article doi))}

% Document starts
\usepackage[utf8]{inputenc}
\usepackage[T1]{fontenc}
\usepackage[english]{babel}
\usepackage{graphicx}
\usepackage{xcolor}
\usepackage{hyperref}
\graphicspath{{images/}{../images/}}
\usepackage{subfiles}
\usepackage[utf8]{inputenc}
\usepackage{graphicx}
\usepackage{comment}
\usepackage{amssymb}
\usepackage{amsmath}

\usepackage{changepage}

 % changed color to make it a bit easier to see

% preamble.
\begin{document}
    \input{supplement_content}

%\subfile{sections/section2}
\bibliographystyle{plain}
\bibliography{references}    
    
\end{document}
